# Supplementary material for: The Longer the Better? The Interplay Between Review Length and Line of Argumentation in Online Consumer Reviews
Source: arXiv:1909.05192 source file (2019-09-26)
Supplement: Supplementary file 1 [file appendix.tex]

\chapter{Source Codes}
  \label{chp:codes}
  \minitoc
  
\section{Classical Lanczos Algorithm}
  \label{sec:matlab:lanczos}

\begin{inlinelisting}{Classical Lanczos as \software{Matlab} code}
     \label{alg:matlab:lanczos}  
  \lstinputlisting[%
    language=Matlab,
    emphstyle=\color{ListingsEmphColor}\bfseries,
    emph={if,for,end},
    deletekeywords={beta,gamma}
  ]{src/UnsymmLanczosBuecker.m}
\end{inlinelisting}
